# Supplementary material for: Intermittency of dynamical phases in a quantum spin glass
Source: arXiv:1907.01609 source file (2019-07-02)
Supplement: Supplementary file 1 [file diagrams-SM.pdf]

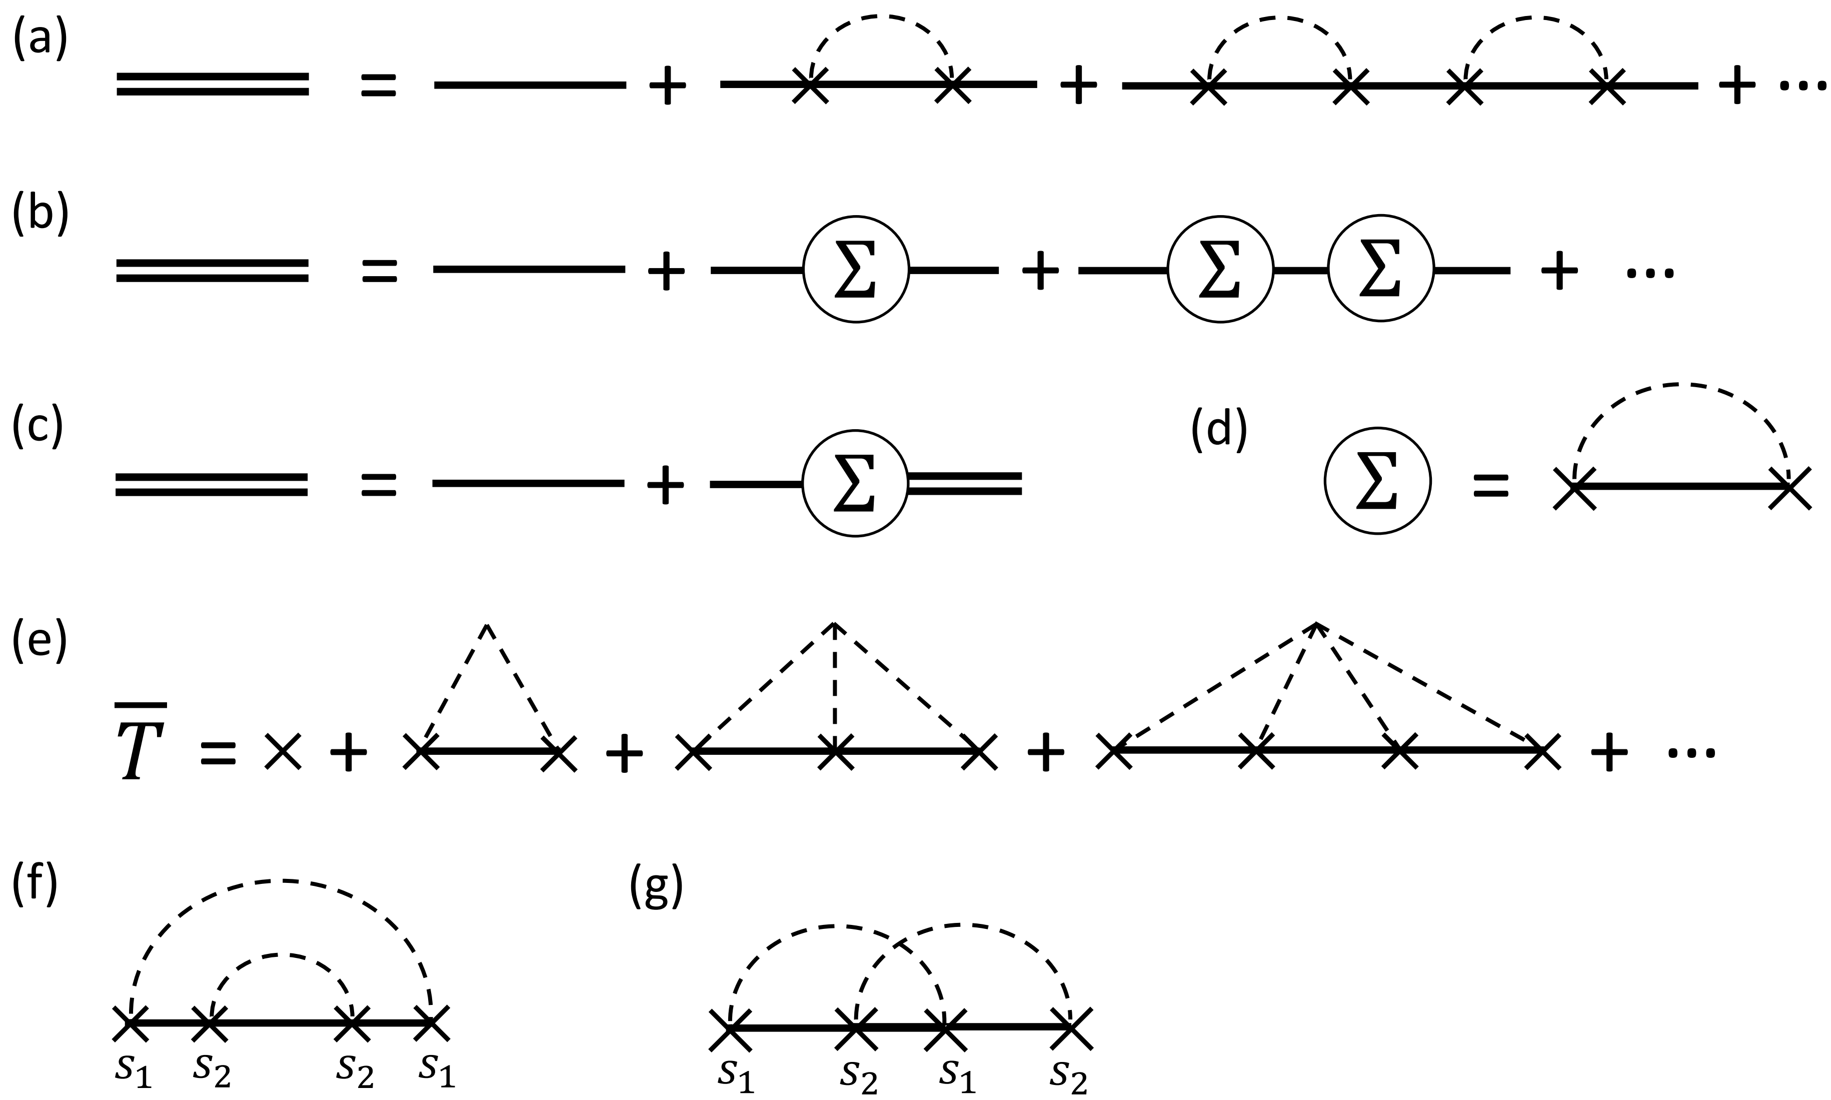
(a)
(b)
(c)
(d)
(e)
$\overline{T}$
(f)
$s_1$ $s_2$ $s_2$ $s_1$
(g)
$s_1$ $s_2$ $s_1$ $s_2$

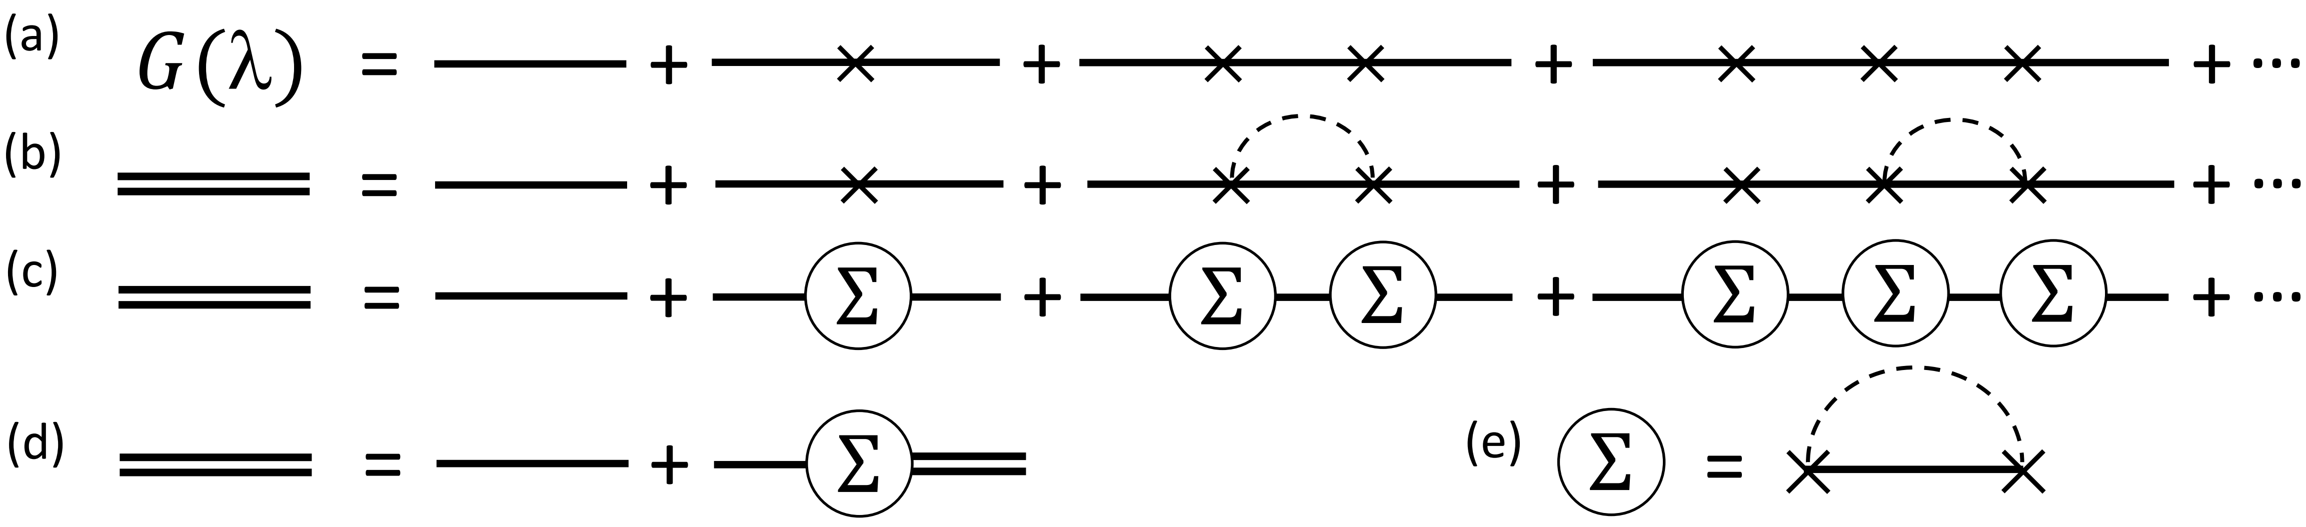
(a)
G(λ)
(b)
(c)
(d)
(e)
Σ

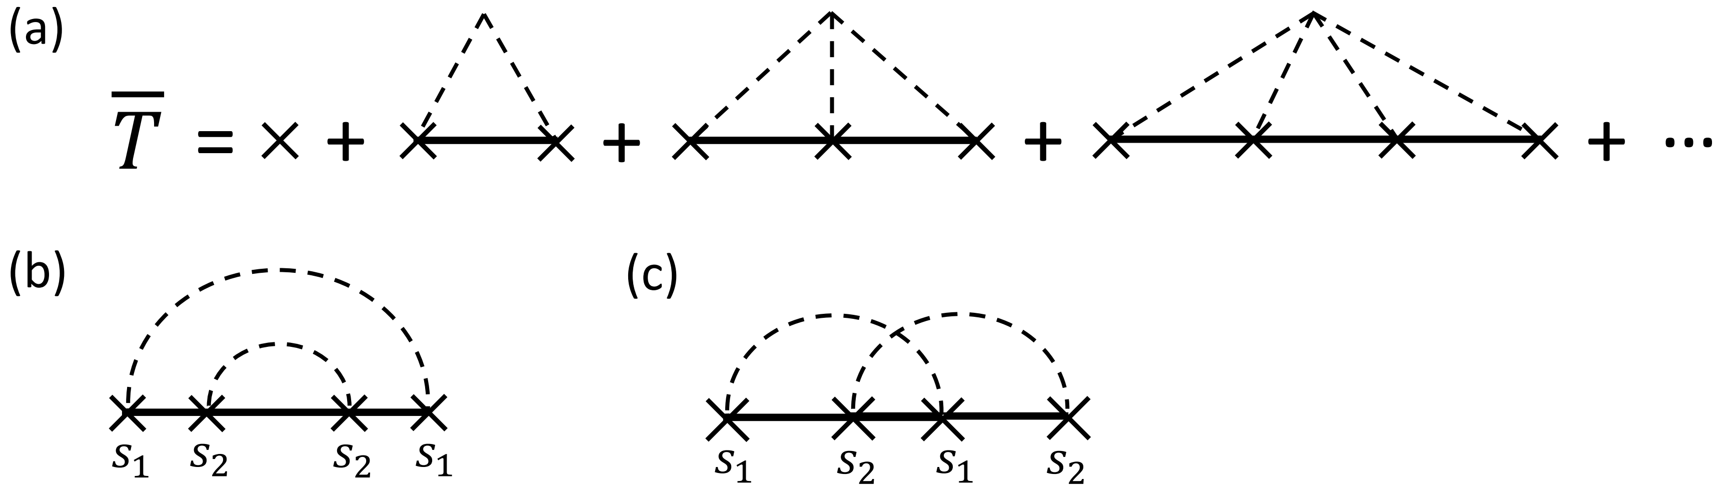
(a)
T̄
(b)
s1 s2 s2 s1
(c)
s1 s2 s1 s2
